# Supplementary material for: Evaluation of OpenAI Codex for HPC Parallel Programming Models Kernel Generation
Source: arXiv:2306.15121 source file (2023-06-27)
Supplement: Supplementary file 1 [file X10.appendix.tex]

\section*{Appendix I}
\label{sec:appendix1}
This section provides pseudocodes for LaRIS's tiled LU factorization and GEMM operation.

\begin{lstlisting}[language=C, caption=LaRIS's tiled LU factorization (GETRF) code., label={lst:getrf_code}]
// Creation of the IRIS graph
iris_graph graph; iris_graph_create(&graph);
iris_task getrf_tasks[TILE_NUM*TILE_NUM], 
    trsm_tasks[TILE_NUM*TILE_NUM], 
    gemm_tasks[TILE_NUM*TILE_NUM*TILE_NUM];
// Tiled LU factorization
for ( int step = 0; step < TILE_NUM; step++ ) {
  // GETRF tasks
  iris_task_create( 
    &getrf_tasks[(step*TILE_NUM)+step]);
  // Dependencies for getrf tasks
  if ( step > 0 ){
    iris_task getrf_depend_tasks[] = 
        { gemm_tasks[((step-1)*TILE_NUM*TILE_NUM)+ 
        ((step*TILE_NUM)+step)] };
    iris_task_depend( getrf_tasks[(step*TILE_NUM) + 
        step], 1, getrf_depend_tasks );
  }
  // Encapsulate GETRF tasks into the graph 
  laris_getrf_graph( graph, 
        getrf_tasks[(step*TILE_NUM)+step], 
        step, step, step, TILE_SIZE, TILE_SIZE, 
        IRIS_Ctile[step*TILE_NUM+step], 
        A_tile[step][step], TILE_SIZE );
  for ( int tile_jj = 1 + step; tile_jj < TILE_NUM; 
        tile_jj++ ) {
    // trsm tasks
    iris_task_create( &trsm_tasks[(step*TILE_NUM)+tile_jj] );
    // Dependencies for trsm tasks
    if ( step == 0 ) {
      iris_task trsm_depend_tasks[] = 
        { getrf_tasks[ ( step * TILE_NUM ) + step ] };
      iris_task_depend( trsm_tasks[(step*TILE_NUM) + 
        tile_jj], 1, trsm_depend_tasks );
    } else {
        iris_task trsm_depend_tasks[] = { 
            getrf_tasks[(step*TILE_NUM)+step], 
            gemm_tasks[((step-1)*TILE_NUM*TILE_NUM)
            +(step*TILE_NUM)+tile_jj]};
        iris_task_depend( trsm_tasks[(step*TILE_NUM) +
            tile_jj], 2, trsm_depend_tasks );
    }
    // Encapsulate trsm tasks into the graph 
    laris_trsm_top_graph( graph, trsm_tasks[(step*TILE_NUM)+ 
          tile_jj], step, step, tile_jj,
          TILE_SIZE, TILE_SIZE, 
          IRIS_Ctile[step*TILE_NUM+step], 
          A_tile[step][step], TILE_SIZE, 
          IRIS_Ctile[step*TILE_NUM+tile_jj], 
          A_tile[step][tile_jj], TILE_SIZE );
  }
  for ( int tile_ii = 1 + step; tile_ii < TILE_NUM;
        tile_ii++ ) {
    // trsm tasks
    iris_task_create( 
        &trsm_tasks[(tile_ii*TILE_NUM)+step] );
    // Dependencies for trsm tasks
    if ( step == 0 ) {
      iris_task trsm_depend_tasks[] = { 
        getrf_tasks[ ( step * TILE_NUM ) + step ]};
        iris_task_depend( trsm_tasks[ ( tile_ii * 
        TILE_NUM ) + step ], 1, trsm_depend_tasks );
    } else {
      iris_task trsm_depend_tasks[] = { 
        getrf_tasks[(step*TILE_NUM)+step], 
        gemm_tasks[((step-1)*TILE_NUM*TILE_NUM)+
        (tile_ii*TILE_NUM)+step] };
      iris_task_depend( 
        trsm_tasks[ ( tile_ii * TILE_NUM ) + step ], 
        2, trsm_depend_tasks );
    }
    // Encapsulate trsm tasks into the graph
    laris_trsm_left_graph( graph, 
        trsm_tasks[(tile_ii*TILE_NUM)+step], 
        step, tile_ii, step, TILE_SIZE, TILE_SIZE, 
        IRIS_Ctile[step * TILE_NUM + step], 
        A_tile[step][step], TILE_SIZE, 
        IRIS_Ctile[tile_ii * TILE_NUM + step], 
        A_tile[tile_ii][step], TILE_SIZE );
    }
    for ( int tile_i = step + 1; tile_i < TILE_NUM; 
            tile_i++ ) {
      for ( int tile_j = step + 1; tile_j < TILE_NUM; 
            tile_j++ ) {
        // gemm tasks
        iris_task_create( &gemm_tasks[(step*TILE_NUM*TILE_NUM) +         
            ((tile_i*TILE_NUM)+tile_j)] );
        // Dependencies for gemm tasks
        if ( step == 0 ) {
          iris_task gemm_depend_tasks[] = { 
            trsm_tasks[(tile_i*TILE_NUM)+step],
            trsm_tasks[(step*TILE_NUM)+tile_j] };
          iris_task_depend(     
            gemm_tasks[(step*TILE_NUM*TILE_NUM)+((tile_i* 
            TILE_NUM)+tile_j)], 2, gemm_depend_tasks );
        } 
        else {
           iris_task gemm_depend_tasks[] = {  
                trsm_tasks[(tile_i*TILE_NUM)+step], trsm_tasks[(step*TILE_NUM)+tile_j],
                gemm_tasks[((step-1)*TILE_NUM*TILE_NUM)+
                ((tile_i*TILE_NUM)+tile_j)] };
           iris_task_depend(    
                gemm_tasks[(step*TILE_NUM*TILE_NUM)+
                ((tile_i*TILE_NUM)+tile_j)], 3, 
                gemm_depend_tasks );
        }
        // Encapsulate gemm tasks into the graph 
        laris_gemm_graph( graph,     
            gemm_tasks[(step*TILE_NUM*TILE_NUM)+
            ((tile_i*TILE_NUM)+tile_j)], step, tile_i,
            tile_j, TILE_SIZE, TILE_SIZE, TILE_SIZE, -1.0, 
            IRIS_Ctile[tile_i*TILE_NUM+step],
            A_tile[tile_i][step], TILE_SIZE, 
            IRIS_Ctile[step*TILE_NUM+tile_j],  
            A_tile[step][ tile_j], TILE_SIZE, 1.0, 
            IRIS_Ctile[tile_i*TILE_NUM+tile_j], 
            A_tile[tile_i][tile_j], TILE_SIZE );
    }
  }
}
iris_graph_submit(graph, iris_default, 1);
\end{lstlisting}

\begin{lstlisting}[language=C, caption=LaRIS's GEMM code., label={lst:gemm_code}]
int laris_gemm_graph( 
    iris_graph graph, 
    iris_task T, 
    int step, int tile_i, int tile_j, 
    int M, int N, int K, 
    TYPE ALPHA, iris_mem d_A, TYPE *h_A, int LDA, 
    iris_mem d_B, TYPE *h_B, int LDB, 
    TYPE BETA, iris_mem d_C, TYPE *h_C, int LDC )
{
  // Memory communication -> input
  iris_task_h2d(T, d_A, 0, M*K*sizeof(TYPE), h_A);
  iris_task_h2d(T, d_B, 0, K*N*sizeof(TYPE), h_B);
  iris_task_h2d(T, d_C, 0, M*N*sizeof(TYPE), h_C);
  // IRIS-BLAS call
  iris_core_nodt_gemm( T, IRIS_BLAS_COL_MAJOR, 
        IRIS_BLAS_NO_TRANS, IRIS_BLAS_NO_TRANS, 
        M, N, K, ALPHA, d_A, LDA, 
        d_B, LDB,BETA, d_C, LDC); 
  // Memory communication -> output
  iris_task_d2h(T, d_C, 0, M*N*sizeof(TYPE), h_C);
  iris_graph_task( graph, T, iris_any, NULL );
  return 0;
}
\end{lstlisting}
